# Supplementary material for: Parameterisation of Reasoning on Temporal Markov Logic Networks
Source: arXiv:2211.16414 source file (2022-11-29)
Supplement: Supplementary file 1 [file supplementary.tex]

% <<< Preamble
%%%%%%%%%%%%%%%%%%%%%%%%%%%%%%%%%%%%%%%%%%%%%%%%%%%%%%%%%%%%%%%%%%%%%%%%%%%%%%%%%%%%%%%%%%%%%%
%%%%%%%%%%%%%%%%%%%%%%%%%%%%%%%%%%%%%%%%%%%%%%%%%%%%%%%%%%%%%%%%%%%%%%%%%%%%%%%%%%%%%%%%%%%%%%
%%%%%%%%%%%%%%%%%%%%%%%%%%%%%%%%%%%%%%%%%%%%%%%%%%%%%%%%%%%%%%%%%%%%%%%%%%%%%%%%%%%%%%%%%%%%%%
%%%%%%%%%%%%%%%%%%%%%%%%%%%%%%%%%%%%%%%%%%%%%%%%%%%%%%%%%%%%%%%%%%%%%%%%%%%%%%%%%%%%%%%%%%%%%%
\documentclass{article}
\pdfpagewidth=8.5in
\pdfpageheight=11in
% The file ijcai22.sty is NOT the same than previous years'
\usepackage{ijcai22}

% Use the postscript times font!
\usepackage{times}

\usepackage{soul}
\usepackage{url}
\usepackage[hidelinks]{hyperref}
\usepackage[utf8]{inputenc}
\usepackage[small]{caption}
\usepackage{graphicx}
\usepackage{amsmath}
\usepackage{booktabs}
\urlstyle{same}

\usepackage{algorithm}
\usepackage{todonotes}
%\urlstyle{same}
\usepackage{tikz}
\usepackage{amssymb}
\usetikzlibrary{shapes,arrows,chains}
\usetikzlibrary[calc]
\usepackage{comment}

\usepackage{placeins}
%\usepackage{float}
%\restylefloat{table}
\definecolor{dartmouthgreen}{rgb}{0.05, 0.5, 0.06}

%\usepackage{amssymb}
%\usepackage{amsmath}
%\usepackage{times}
%\newtheorem{postulate}{Principle}
%\newtheorem{notation}{Notations}

%\newtheorem{lemma}{Lemma}

%\newtheorem{conjecture}{Conjecture}

%%%%%%%%%%%%%%%%%%%%%%%%%%%%%%%%%%%%%%%%%%%%%%%%%%%%%%%%%%%%%%%%%%%%%%%%%%%%%%%%%%%%%%%%%%%%%%
%%%%%%%%%%%%%%%%%%%%%%%%%%%%%%%%%%%%%%%%%%%%%%%%%%%%%%%%%%%%%%%%%%%%%%%%%%%%%%%%%%%%%%%%%%%%%%
%%%%%%%%%%%%%%%%%%%%%%%%%%%%%%%%%%%%%%%%%%%%%%%%%%%%%%%%%%%%%%%%%%%%%%%%%%%%%%%%%%%%%%%%%%%%%%
%%%%%%%%%%%%%%%%%%%%%%%%%%%%%%%%%%%%%%%%%%%%%%%%%%%%%%%%%%%%%%%%%%%%%%%%%%%%%%%%%%%%%%%%%%%%%%	

%\newcommand{\bigsig}{ $\Large$ \sigma $\normalsize$ }

%%%%%%%%%%%%%%%%%%%%%%%%%%%%%%%%%%%%%%%%%%%%%%%%%%%%%%%%%%%%%%%%%%%%%%%%%%%%%%%%%%%%%%%%%%%%%%
%%%%%%%%%%%%%%%%%%%%%%%%%%%%%%%%%%%%%%%%%%%%%%%%%%%%%%%%%%%%%%%%%%%%%%%%%%%%%%%%%%%%%%%%%%%%%%
%%%%%%%%%%%%%%%%%%%%%%%%%%%%%%%%%%%%%%%%%%%%%%%%%%%%%%%%%%%%%%%%%%%%%%%%%%%%%%%%%%%%%%%%%%%%%%

\pdfinfo{
/TemplateVersion (IJCAI.2022.0)
}

\title{Supplementary material for\\  Parameterisation and Principles of Reasoning on \\ Temporal Markov Logic Networks}

\author{
    Anonymous submission to IJCAI22.}

\begin{document}
	
% <<< abstract
%
\maketitle  

\input{appendix.tex}
%\end{appendix}

% >>>

\end{document}
